# Supplementary material for: Two methods to analyse radial diffusion ensembles: the peril of space- and time- dependent diffusion
Source: arXiv:2407.04669 source file (2024-09-04)
Supplement: Supplementary file 1 [file supplementary.pdf]

# Supplementary Information for “Two methods to compare radial diffusion ensembles: the peril of space- and time- dependent diffusion”

August 13, 2024

## List of Figures

|    |                                                                                               |    |
|----|-----------------------------------------------------------------------------------------------|----|
| S1 | Time to monotonicity for initial condition parameters. . . . .                                | 2  |
| S2 | Time to monotonicity for initial condition parameters (Alternative view) . . . . .            | 3  |
| S3 | $\mathcal{N}$ and $\mathcal{N}_t$ . . . . .                                                   | 4  |
| S4 | $\mathcal{E}$ and $\mathcal{E}_t$ . . . . .                                                   | 5  |
| S5 | Time to monotonicity for initial condition parameters, with loss. . . . .                     | 6  |
| S6 | Time to monotonicity for initial condition parameters, with loss. (Alternative view). . . . . | 7  |
| S7 | $\mathcal{N}$ and $\mathcal{N}_t$ , with loss. . . . .                                        | 8  |
| S8 | $\mathcal{E}$ and $\mathcal{E}_t$ , with loss. . . . .                                        | 9  |
| S9 | (Same as Fig 11) Comparing phase space density for $L_{outer} = 6.5$ vs $7.5$ . . . . .       | 10 |

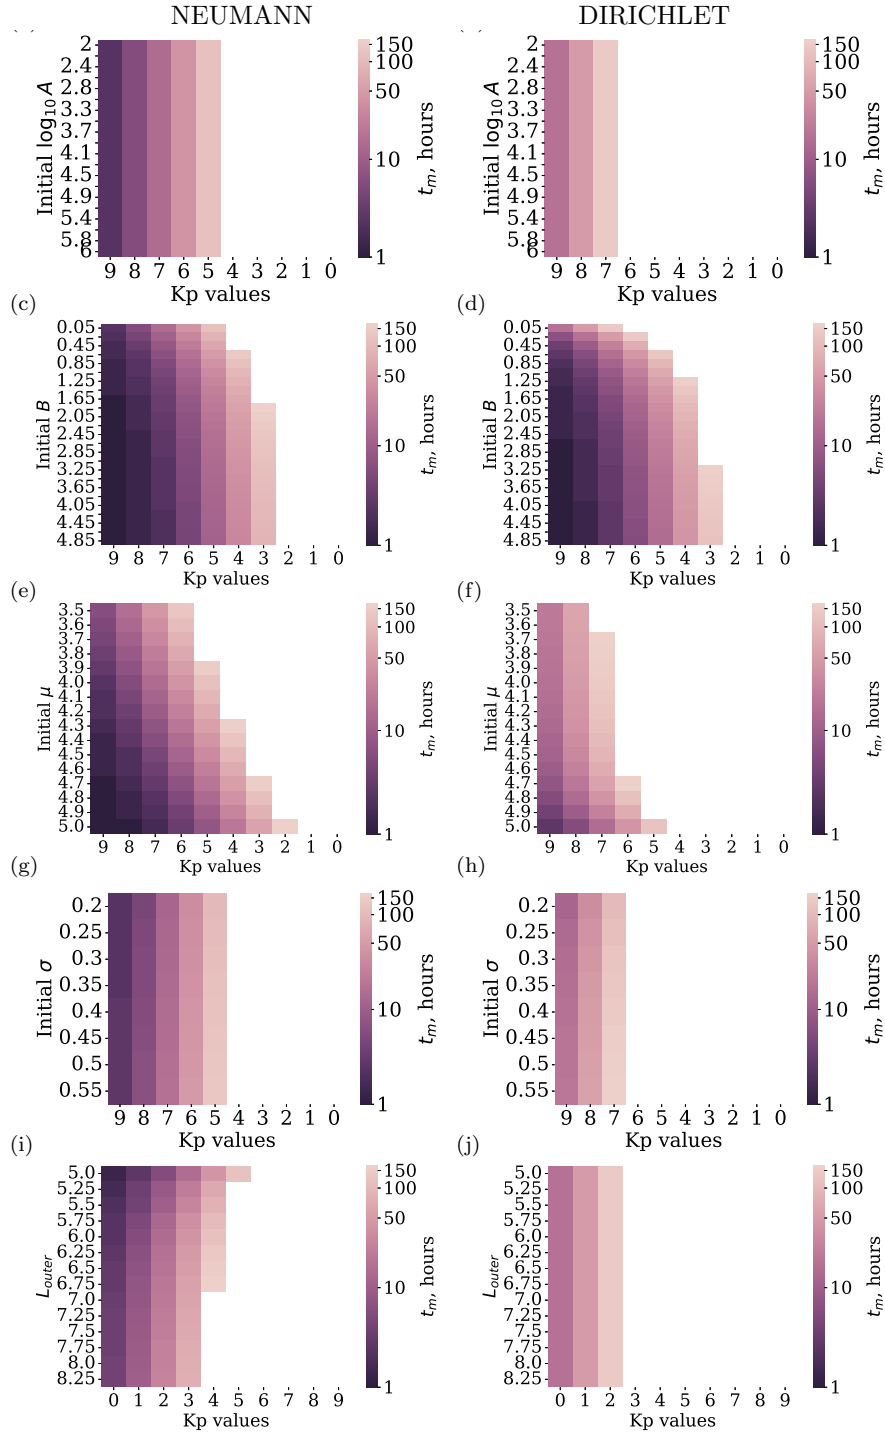

Figure S1: Time to monotonicity at constant Kp for all parameters varied in our initial conditions analysis. The left column corresponds to experiments with a Neumann (fixed gradient) outer boundary condition, and the right column to a Dirichlet (fixed value) outer boundary condition.

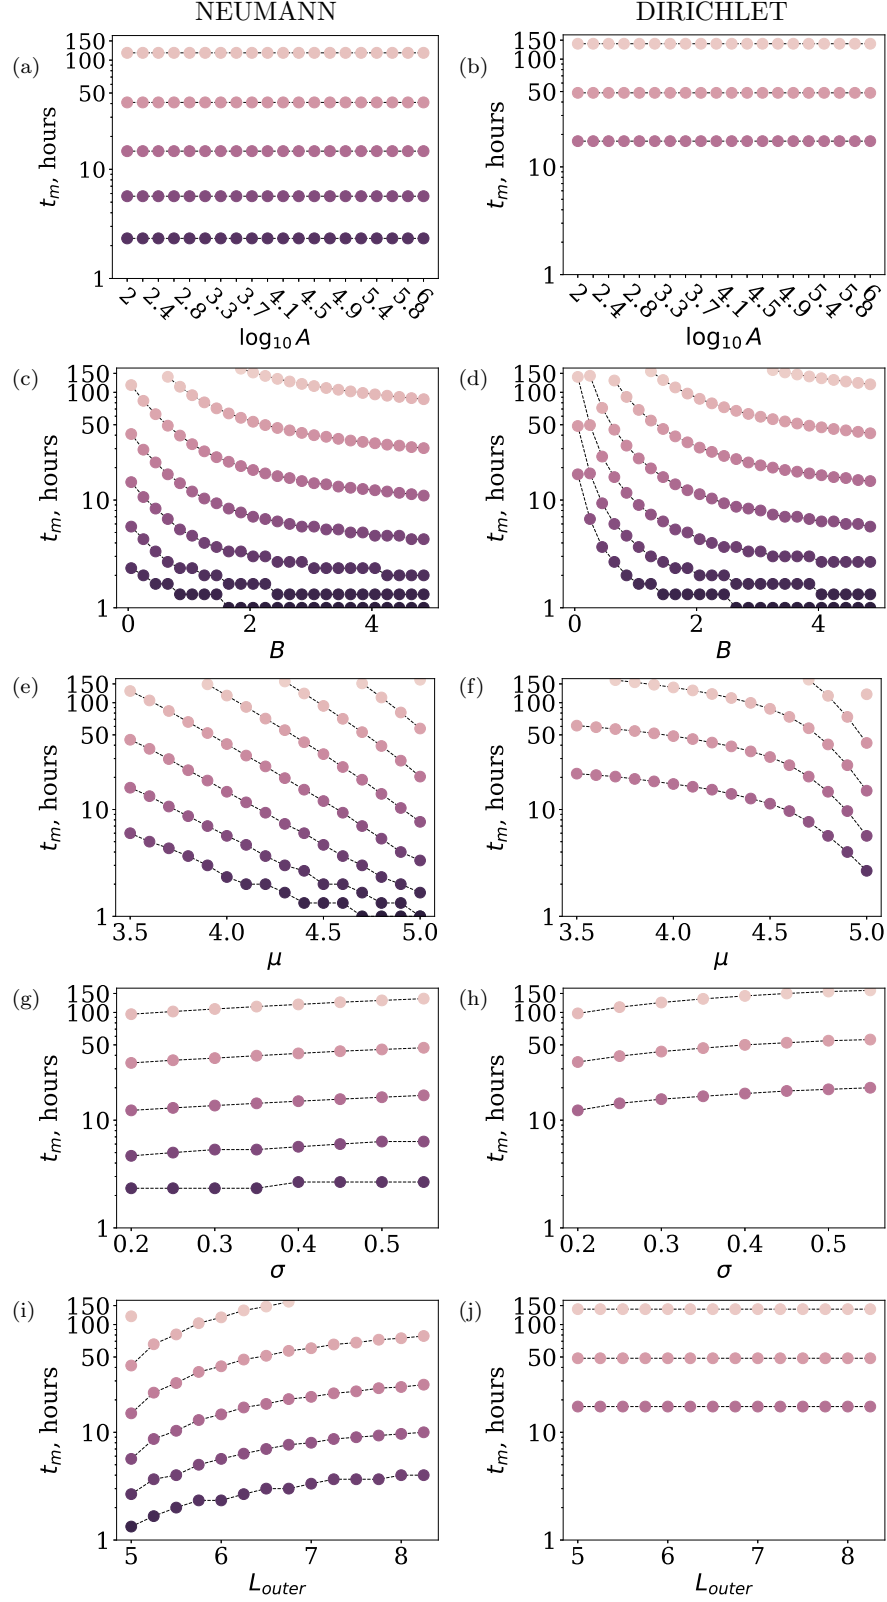

Figure S2: Time to monotonicity at constant Kp for all parameters varied in our initial conditions analysis. The left column corresponds to experiments with a Neumann (fixed gradient) outer boundary condition, and the right column to a Dirichlet (fixed value) outer boundary condition. Each line corresponds to the  $t_m$  found at a given Kp value, as the parameter (e.g.  $B, \mu$  etc.) varies. The bottom line in each plot corresponds to Kp= 9 from Figure S1, and higher lines correspond to Kp= 8, 7 etc. Alternative depiction of S1; the coloured markers simply reflect the  $t_m$  value (i.e. the y-axis) to aid joint analysis with Figure S1.

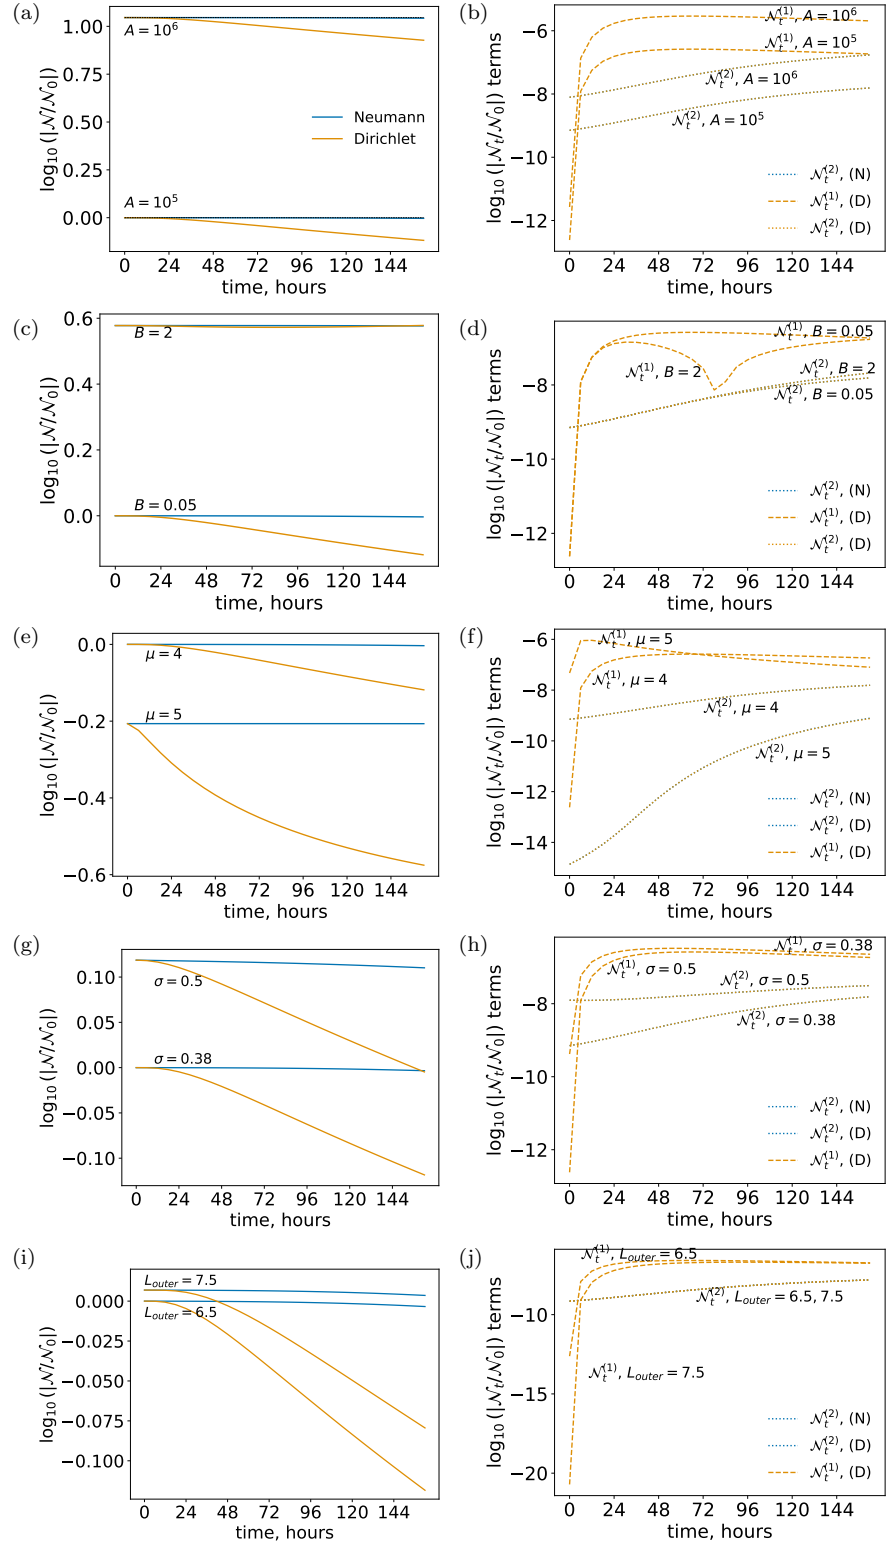

Figure S3:  $\mathcal{N}$  analysis for each parameter, for one week, compared to the default Neumann and Dirichlet values. Left:  $\mathcal{N}$  values. Right: Component terms  $\mathcal{N}_t$ . Here, all results are included for completeness; selected results (including easier to interpret subsets of all the  $\mathcal{N}_t$  components) can be found in the main text.

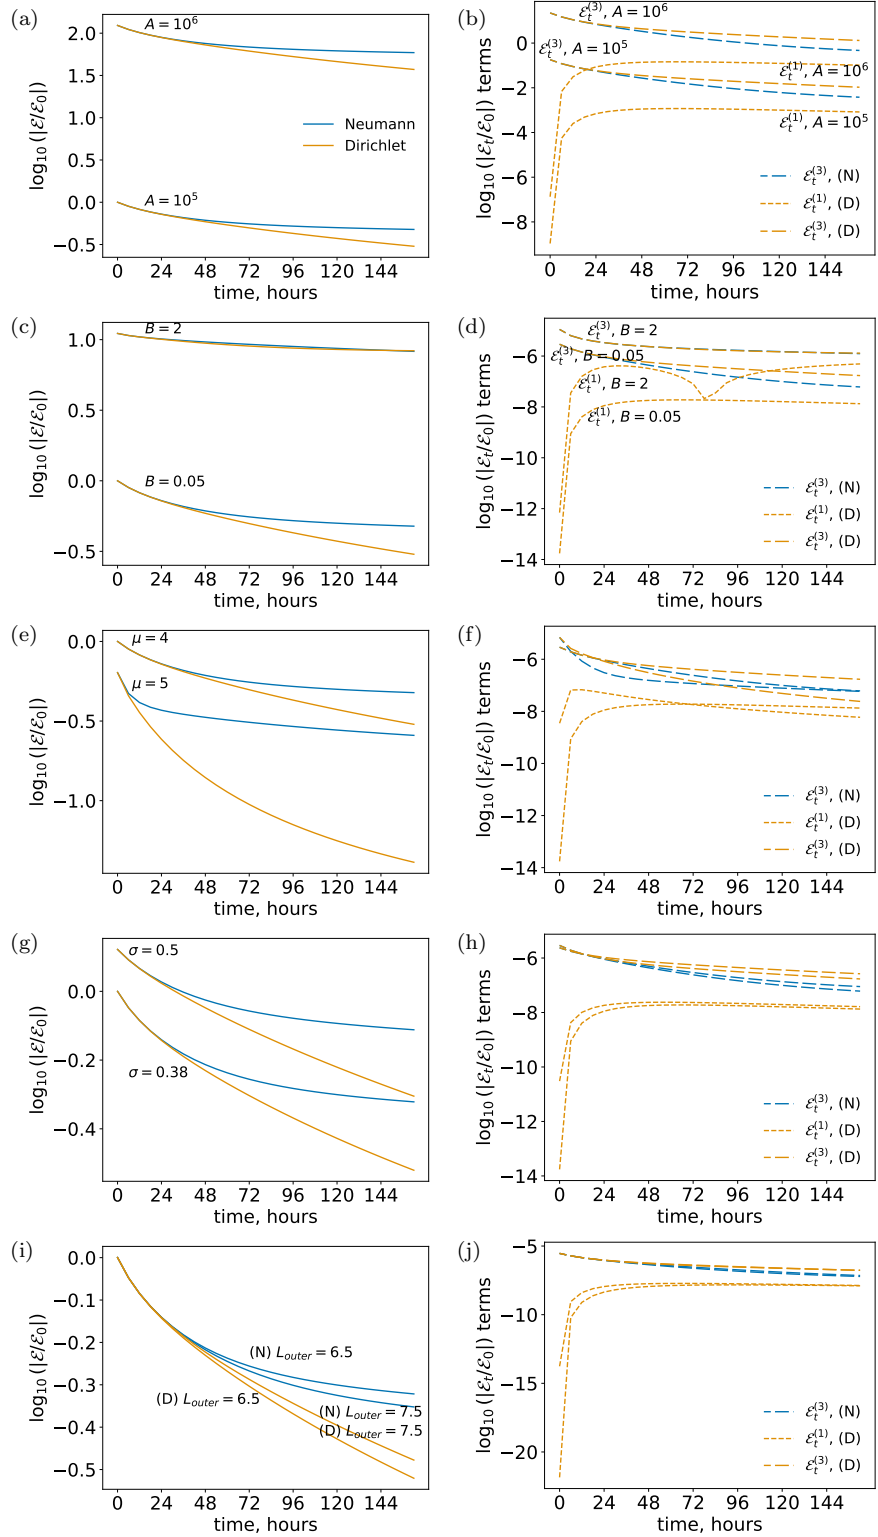

Figure S4:  $\mathcal{E}$  analysis for each parameter, for one week, compared to the default neumann and Dirichlet values. Left:  $\mathcal{E}$  values. Right: Component terms  $\mathcal{E}_t$ . Here, all results are included for completeness; selected results (including easier to interpret subsets of all the  $\mathcal{E}_t$  components) can be found in the main text.

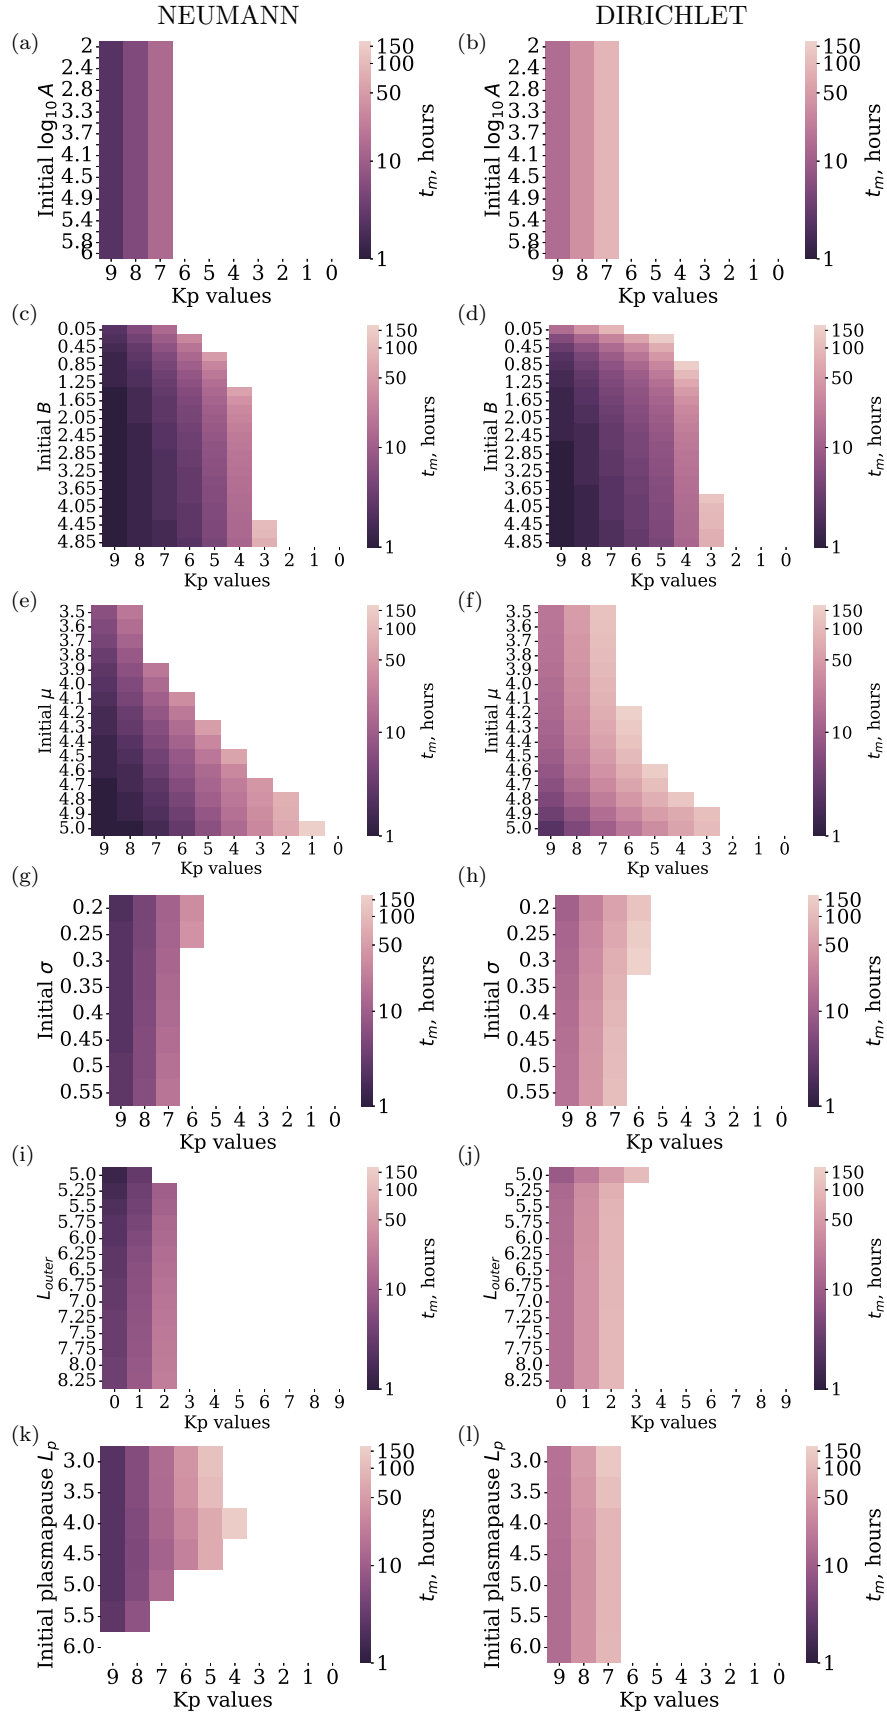

Figure S5: Time to monotonicity at constant Kp for all parameters varied in our initial conditions analysis, with loss from pitch angle scattering included. The left column corresponds to experiments with a Neumann (fixed gradient) outer boundary condition, and the right column to a Dirichlet (fixed value) outer boundary condition.

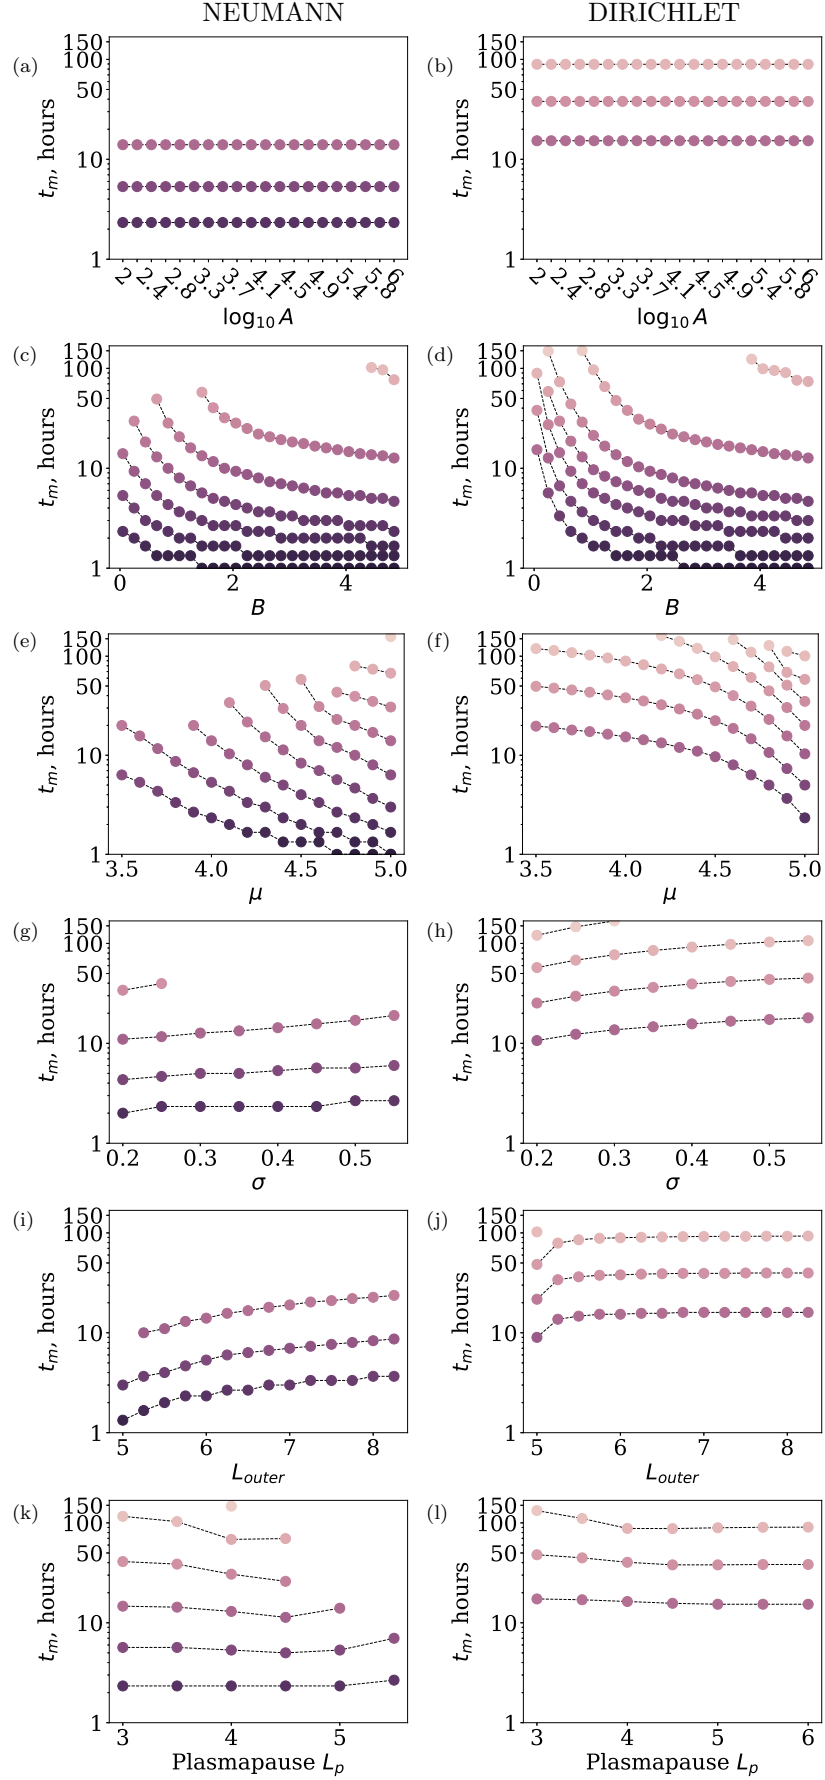

Figure S6: Time to monotonicity at constant  $K_p$  for all parameters varied in our initial conditions analysis, with loss from pitch angle scattering included. Left column: Neumann (fixed gradient) outer boundary condition. Right column: Dirichlet (fixed value) outer boundary condition. Each line corresponds to the  $t_m$  found at a given  $K_p$  value, as the parameter (e.g.  $B, \mu$  etc.) varies. The bottom line in each plot corresponds to  $K_p=9$  from Figure S1, and higher lines correspond to  $K_p=8, 7$  etc. Alternative depiction of S5; the coloured markers simply reflect the  $t_m$  value (i.e. the y-axis) to aid joint analysis with Figure S5.

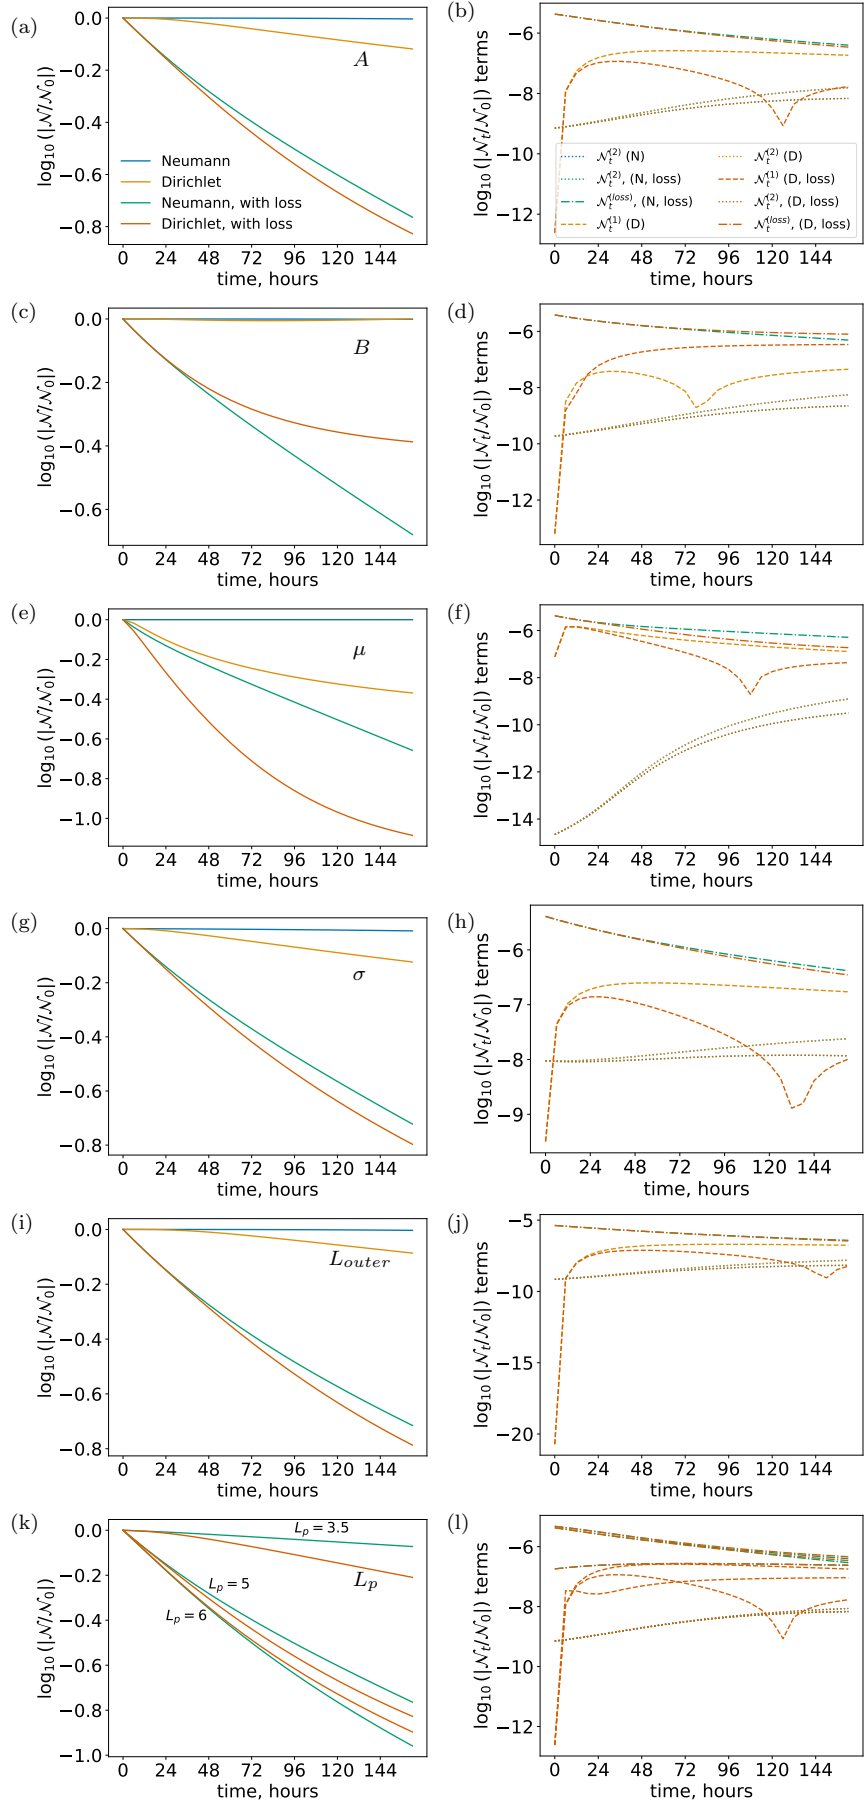

Figure S7:  $\mathcal{N}$  analysis for each parameter, for one week, compared to the same parameter values without loss  $\mathcal{L}$ . Left:  $\mathcal{N}$  values. Right: Component terms  $\mathcal{N}_t$ . Here, all results are included for completeness; selected results (including easier to interpret subsets of all the  $\mathcal{N}_t$  components) can be found in the main text.

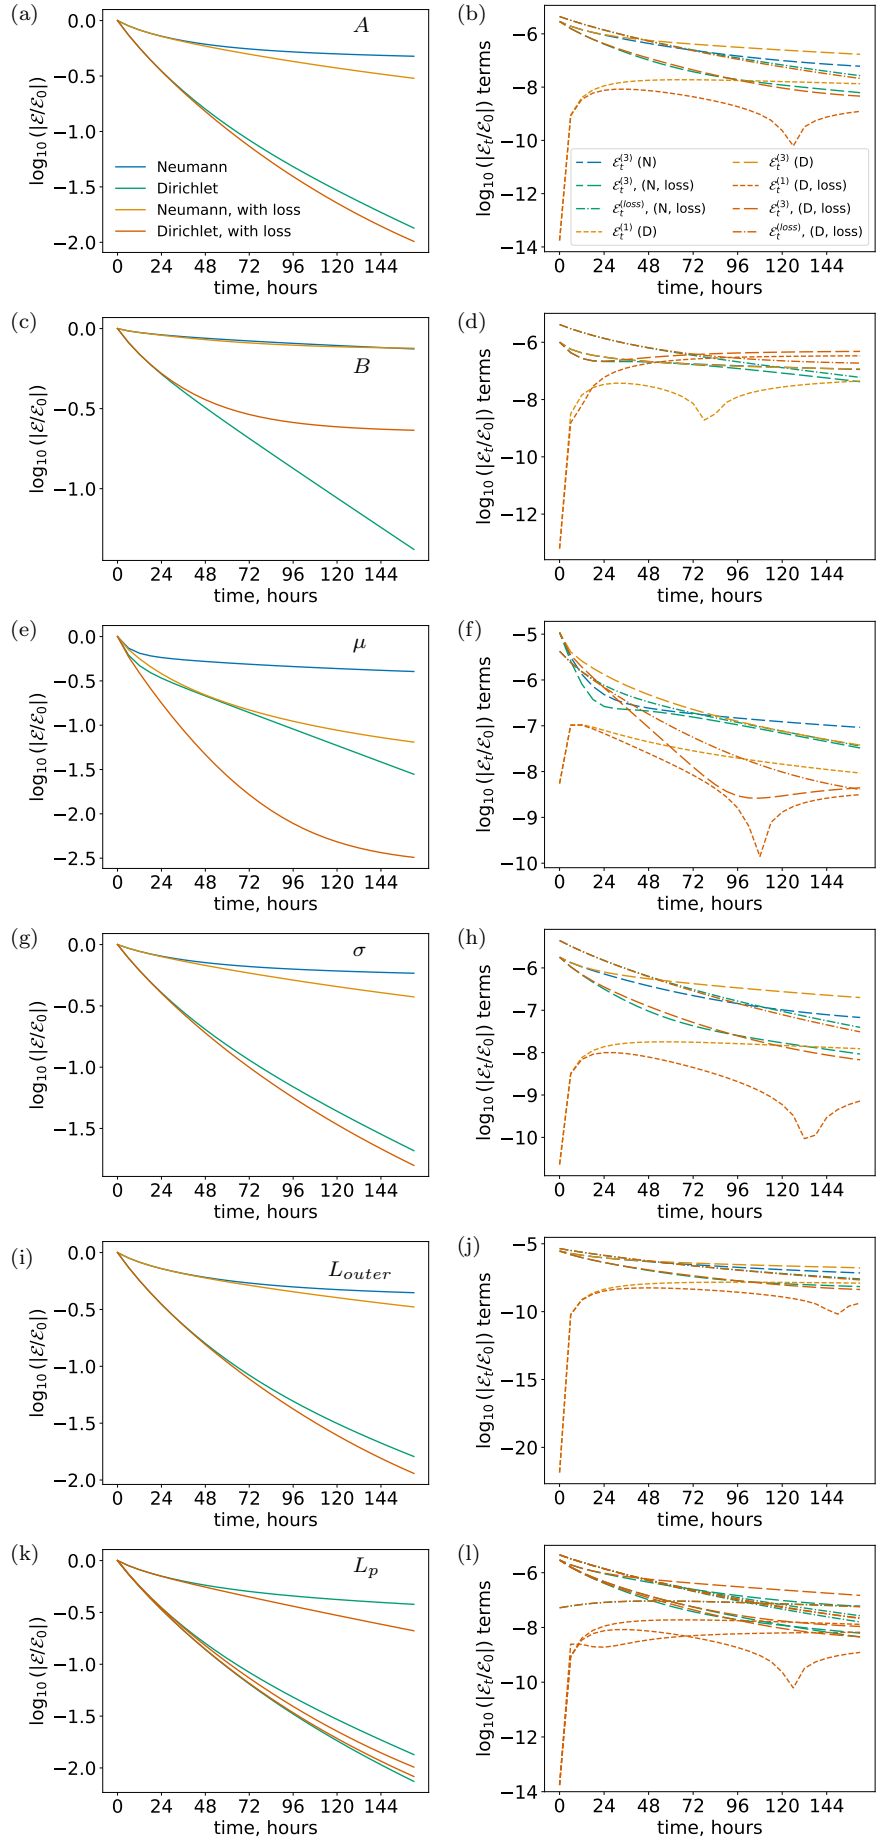

Figure S8:  $\mathcal{E}$  analysis for each parameter, for one week, compared to the same parameter values without loss  $\mathcal{L}$ . Left:  $\mathcal{E}$  values. Right: Component terms  $\mathcal{E}_t$ . Here, all results are included for completeness; selected results (including easier to interpret subsets of all the  $\mathcal{E}_t$  components) can be found in the main text.

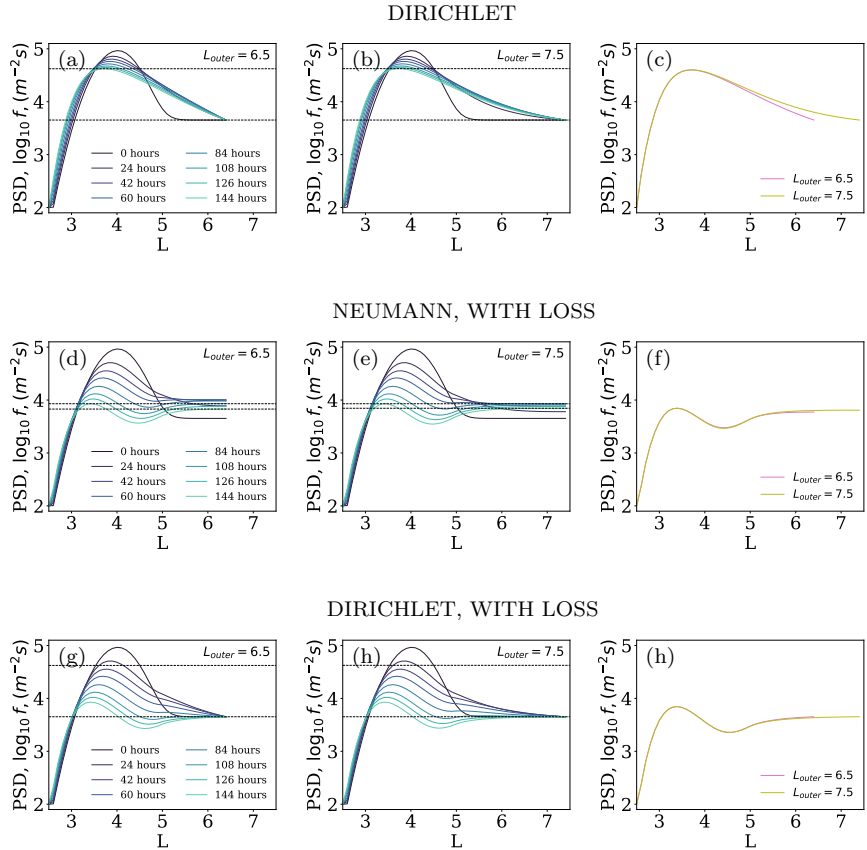

Figure S9: Comparing the effect of varying the outer boundary locations: snapshots of phase space density throughout week-long simulations, in a similar style to Figure 11 but for Dirichlet outer boundary conditions (OBC) without loss (Row 1), Neumann OBC with loss (Row 2) and Dirichlet OBC with loss (Row 3). The first column shows these snapshots of PSD when the outer boundary is set at  $L_{outer} = 6.5$  whilst the second column shows the snapshots with an outer boundary at  $L_{outer} = 7.5$ . Dotted lines indicate the height of the peak and plateau by the end of the week. The third column compares the final PSD profiles at the end of the week for both outer boundary locations.
